# Supplementary material for: Logit Attenuating Weight Normalization
Source: arXiv:2108.05839 source file (2021-08-12)
Supplement: Supplementary file 1 [file isolated.tex]

\documentclass{article}
\usepackage[utf8]{inputenc}
\usepackage{url}

\usepackage[ruled, lined, linesnumbered]{algorithm2e}

\usepackage{url}
\usepackage{amsthm, amsmath, amsfonts, amssymb}

\newcounter{mycounter}
\stepcounter{mycounter}

\title{Fully Homogeneous Nets: Isolatedness of LAWN's Constrained Optima}

\author{}
\date{June 3, 2021}

\begin{document}

\maketitle

\def\lag{{\cal{L}}}

Let $w=\{w^\ell\}$, $w\in R^n$. Consider the optimization problem solved in the constrained phase of LAWN:
\begin{equation}
    min_w \; L(w)  =  -\frac{1}{m}\sum_{i=1}^m \log p_{y_i}(w) \mbox{ s.t. } \|w^\ell\|^2 = s^\ell \; \forall \ell \label{eq:1}
\end{equation}
Let us assume that $L$ is a twice continuously differentiable function of $w$. We are interested in the minima of (\ref{eq:1}). The minima is a subset of the KKT points of (\ref{eq:1}). Let $\lag$ denote the lagrangian,
\begin{equation}
    \lag(w,\lambda) = L(w) + \sum_\ell \lambda_\ell (\|w^\ell\|^2 - s^\ell) \label{eq:2}
\end{equation}
$w$ (combined with a $\lambda$) is a KKT point of (\ref{eq:1}) if
\begin{equation}
    \nabla_w \lag(w,\lambda) = 0 \mbox{ and } \|w^\ell\|^2 = s^\ell \; \forall \ell \label{eq:3}
\end{equation}
There is usually a bit of technicality associated with connecting minima with KKT points. That technicality turns out to be a non-issue for (\ref{eq:1}). To clarify this, we formally state a lemma.

{\bf Lemma 1.} Every minimum of (\ref{eq:1}) is necessarily a KKT point of (\ref{eq:1}). $\qedsymbol$

\def\wtilde{\tilde{w}}

{\bf Proof of Lemma 1.} In general, a minimum is a KKT point if a regularity condition (aka constraint qualification) is satisfied. There are several sufficiciency conditions that imply regularity. One of them, that suffices our purpose here is: the gradients of the equality constraints are linearly independent at the point $w$ that is tested. In our case, the gradients are $\{2\wtilde^\ell\}$ where $\wtilde^\ell$ is a full vector with $w^\ell$ in the $\ell$-th subvector and $0$ for all other subvectors. Since each $w^\ell\not= 0$ and the vectors in $\{2\wtilde^\ell\}$ are pairwise orthogonal, the linear independence condition holds, thus implying the regularity condition.

Roughly, we say that a property holds in {\it general position} if it holds for almost all tiny random perturbations of data. The property that we are interested is {\it isolatedness of KKT points}. A KKT point $w$ is {\it isolated} if there is an open neighorhood of $w$ in which there is no other KKT point. 
To prove that isolatedness holds in general position, we need to introduce data perturbations. Let us perturb the loss function, $L$ as
\begin{equation}
    L(w)  =  -\frac{1}{m}\sum_{i=1}^m \log p_{y_i}(w) \; + \; \epsilon^T w \label{eq:4}
\end{equation}
where $\epsilon$ is a vector that lies in the tiny open set,
\begin{equation}
    E = \{ \epsilon : \|\epsilon\| < \delta \} \label{eq:5}
\end{equation}
where $\delta$ is chosen to be any small, but positive real number. Now let us consider the KKT points of (\ref{eq:1}) with $L$ defined using (\ref{eq:4}).

{\bf Theorem 1.} For almost all choices of $\epsilon\in E$, the set of KKT points of (\ref{eq:1}) is isolated and finite.

{\bf Proof of Theorem 1.} The proof uses the Transversality theorem, a corollary of Sard's theorem of differential topology~[1].

\def\Ytil{\tilde{Y}}

{\bf Transversality theorem} Suppose $F: Y\times Z \to R^N$ is a smooth differentiable function such that (a) $Y$ and $Z$ are open sets in $R^L$ and $R^M$ and (b) the jacobian of $F$ with respect to $(y,z)$ has full row rank for all $(y,z)\in Y\times Z$. Then 
%for almost all $z\in Z$, 
in general position, i.e., for almost all $z\in Z$,
the set $\Ytil(z) = \{ y\in Y : F(y,z) = 0 \}$ is either empty or a differentiable manifold of dimension $(L-N)$. $\qedsymbol$

Now let us set up the KKT points determination as an instance of a set of equations, $F(y,z)=0$.
Let $y=(w,\lambda)\in R^{n+l}$ where $n$ is the dimension of $w$ and $l$ is $\#\ell$. Let $z=\epsilon$. Let $F(y,z)=0$ consist of the following equation sets that define a KKT point (see (\ref{eq:3})): $\nabla_w \lag(w,\lambda) = 0$, $\|w^\ell\|^2 - s^\ell = 0 \; \forall \ell$. With $(y,z)=(w,\lambda,\epsilon)$, we can simply look at the sub-Jacobian of $F$ with respect to $\epsilon$ and the $w^\ell$ to verify that Jacobian of $F$ with respect to $(y,z)$ has full row rank. (Note in particular: $\nabla_w \lag(w,\lambda)$ has $\epsilon$ and so its jacobian with respect to $\epsilon$ is the identity matrix; also, the jacobian of $\|w^\ell\|^2 - s^\ell$ with respect to $w^\ell$ is $2w^\ell$ which is non-zero.)

Therefore transversality theorem applies. For our problem, $L=n+l$, $M=n$ and $N=n+l$. Since $L=N$, transversality theorem implies that the set of KKT points, i.e., the set of solutions of $F(y,z)=0$, is a zero dimensional manifold.\footnote{The set is non-empty because, in the compact set defined by the equalities, there has to be at least one minimum and one maximum.} A zero-dimensional manifold, by definition, is isolated. In addition, $w$ lies in a bounded set (due to the equality constraints). It can also be shown (details to be written) that $\lambda$ also lies in a bounded set. This implies that the set of KKT points is not only a zero dimensional manifold, but it is also compact. These together imply that the set of KKT points is finite, which is stronger than saying that it is isolated.

By Lemma 1, the set of minima is a subset of the set of KKT points, and so it is also isolated and finite.

\vspace*{0.5cm}

{\Large\bf References}

\vspace*{0.2cm}

[1] V. Guillemin and A. Pollack. {\em Differential Topology}. Prentice-Hall, 1974.

\end{document}
