# Supplementary material for: Logit Attenuating Weight Normalization
Source: arXiv:2108.05839 source file (2021-08-12)
Supplement: Supplementary file 2 [file natureofoptima.tex]

\section{Nature of Optima}
\label{sec:optima}

Let us start by defining a manifold. A manifold is a nonlinear surface with a dimension. In 3d, i.e., $w\in R^3$, if we have a single equation, e.g., $w_1^2 + w_2^2 + w_3^2 = 1$, it is a surface, or {\em a manifold of dimension $2$}: the single constraint removes one degree of freedom. If we include one more equation, say, $w_1+w_2+w_3 = 0.5$ we get a curve, or, equivalently, {\em a manifold of dimension $1$}: two constraints remove two degrees of freedom. If we include a third constraint, say $w1=0.1$, then we get an isolated set of points\footnote{Even in the case of positive dimensional manifolds, there can be many disconnected components.}, or equivalently, a {\em a manifold of dimension $0$}. In general if $w\in R^n$, and $h(w)=0$ is a set of $m$ equations, then the resulting set is {\em a manifold of dimension $(n-m)$.} When the manifold dimension is positive, we will refer to it as a {\em continuum}.

Let $w\in R^n$ and there be $m$ training examples. Let us mainly focus on over-parametrized networks, for which $n\gg m$. For the $i$-th training example let $p_{y_i}(w)$ denote the probability assigned by the network to the target class $y_i$. 

{\bf Toy example.} Consider a linear classifier with two inputs and no bias, with scoring function $w_1x_1 + w_2x_2$, and a pair of symmetric training examples, $(2,1)$ belonging to the positive class and $(-2,-1)$ belonging to the negative class. (Though there are two examples, since they are symmetric, it is as if there is just one example. Seen another way, the losses of the two examples are identical.) While any $w$ with $2w_1 + w_2 > 0$ will give perfect classification, the max margin direction, $w=(2,1)$ will give the most robust (and hence, possibly the best generalizing) solution.

From Subsection~\ref{subsec:curradloss} let us recall the following loss functions: $L_{Normal}$, $L_{LSR}$, $L_{Flooding}$, and $L_{L2}$ (see  (\ref{eq:Normal})-(\ref{eq:L2})). Figure~\ref{fig:contours} shows the contours of these loss functions and various properties of the four methods for the Toy example.

{\bf LSR Training.} 
For a given $i$ the least value of $L_{LSR}$ occurs when $p(w;i)=q(i)$. In over-parametrized networks, it is easy to achieve a perfect minimum in which loss is minimized for each $i$. Therefore, the LSR minima are given by
\begin{equation}
    p_{k}(w;i) = q_{k}(i) \;\; \forall\; k=1,\ldots,nc, \;\; i=1,\ldots,m
\end{equation}
For each i, one of the $nc$ equations over index $k$ is redundant because $\sum_k p_{k}(w;i) = \sum_k q_{k}(i) = 1$. Thus, the set of minima of $L_{LSR}(w)$ is a continuum: a manifold of dimension $(n-m(nc-1))$. As Figure~\ref{fig:contours} shows for the toy example, the max margin solution will be obtained only if the weight initialization is carefully chosen.

\begin{figure*}
    \includegraphics[width=\textwidth]{images/natureopt.jpg}
    \caption{Contours of $L_{LSR}$, $L_{Flooding}$, $L_{L2}$ and $L_{Normal}$ and behaviors of gradient descent on the Toy example. For $LSR$ and $Flooding$, the set of optima is a line, which is a manifold of dimension 1. Different weight initializations (two cases, $A$ and $B$ are shown) lead to different final weights. Though these weights correspond to perfect classification, they are not margin maximizing. The max margin solution will be obtained only if the initialization is specially done (e.g., started from $(0,0)$). For $Normal$, the minima exist at infinity, and, for any starting point, e.g., C in the plot, gradient descent asymptotically (five weight vectors along the path are shown) moves weights to infinity, zeroes out the effect of the initial condition and gets the max margin direction (implicit bias). In this example, $L2$ and $LAWN$ find the max margin directions; in general, they find good approximations to the max margin direction.}
    \label{fig:contours}
\end{figure*}

{\bf Flooding Training.} 
With an over-parametrized network, $L_{Flooding}(w)$ can be made perfectly zero. Since this is a single equation in $n$ weight variables, the set of optima is a manifold of dimension $(n-1)$. Again, as in the LSR case, we have a continuum of optima (in fact, the dimension of the optima manifold for flooding is generally higher than that of LSR).

{\bf Normal Training.} 
In this case, the perfect minima exist at infinity. In terms of directions, the set of optima can be thought of as a manifold of dimension $(n-m)$ that moves to infinity. (The above statement needs to be rewritten.) Implicit bias dictates that, among the manifold continuum of choices, gradient descent will asymptotically choose local max margin directions which are isolated.

We are generally used to thinking that the optima in weight space (where some training loss is minimized) is an isolated set of points, i.e., a manifold of dimension 0. But, as we see above, it is true only in some cases. In general, it is a continuum. 

Also, the set of optima can have many disconnected components, with each component being a connected manifold. Each component has a basin of attraction - the set of all starting points of an optimizer (say, gradient descent flow) that will lead to one of the optima in the component. While the symmetry associated with neuronal rearrangement within any layer can lead to the formation of these components, there can also exist components that are fundamentally different from each other - Think of different ways of separating classes perfectly using the same given deep net architecture. These components can have quite different generalization properties; In some, the loss can vary sharply leading to not-so-good generalization and in other components the loss can be flat and yielding good generalization. 

Further, even within one optima component, different optima can have different generalization/loss sharpness-flatness properties. In the toy example, a weight vector satisfying $w_2 = 2w_1$ is the max margin solution, hence robust and possibly an excellent generalizing direction. On the other hand, weight vectors on the line $2w_1+w_2=c$ with $w_1$ and $w_2$ becoming large in magnitude may be poor in generalization since they tend towards zero margin. 

The noise in the stochastic optimizer combined with suitable learning rate scheduling - see the appendix on escape - can help training (a) to escape basins of components with sub-optimal generalization and (b) after reaching a good basin, to go to the right optima with the best generalization. On a real deep net solution (CIFAR10), Sagun et al~\cite{Sagun2017} (see subsection 4.1 and Figure 8 there) point to how decreasing the batch size leads to the finding of a better generalizing optimum within the same basin of attraction.

As we saw earlier for LSR and Flooding, with vanilla (full batch) gradient descent, different initializations lead to different optima. This result does not change even if we use sgd.  In the case of Normal training, the optima are at infinity, so the solution goes to infinity, the effect of the initialization gets diminished, and hence we asymptotically obtain the max margin direction. See Figure~\ref{fig:ImpBias}. This is the implicit bias result which LSR and Flooding do not enjoy. The loss of implicit bias helping generalization is an issue with methods such as LSR and Flooding.

{\bf L2 Regularization.}
Because of the addition of a strongly smooth regularization function, the optima of $L_{Reg}$ is a set of isolated points. In the toy example, irrespective of $\rho$, these optima are along the max margin direction. In general, as $\rho$ increases from zero to high values, an optimum moves away from a max margin solution. Tuning $\rho$ gives good generalization. In a later discussion we can say how LAWN is related, but even better due to finer, layer-wise regularization.

{\bf To Add:} Some problems that are unresolved which can be opened up as new directions, especially, the nature of optima (isolated or continuum) in non-homogeneous nets, and also how implicit bias works for them.
