# Supplementary material for: Logit Attenuating Weight Normalization
Source: arXiv:2108.05839 source file (2021-08-12)
Supplement: Supplementary file 3 [file logisticbenefit.tex]

\section{Logistic based margin approximation}
\label{sec:logisticbenefit}

The smooth approximation of the margin ((\ref{eq:normmarginmax}) and (\ref{eq:constrmaxmargin})) by the logistic or cross entropy functions ((\ref{eq:appnormmarginmax}) and (\ref{eq:constropt})) can possibly even have properties that are better than margin maximization.
When the training set has a noisy example of one class that is in the middle of a region of another class and over-parametrization causes an overfitting region (an undesired hole) to be formed around the noisy point, the logistic and cross entropy approximations can reduce the size of this region. Figure~\ref{fig:LogisticBetterness} demonstrates this via an example. This happens due to these losses pushing the boundary closer to the locally minority class. \keerthi{Keerthi and Sirou to work on adding more blue points to the figure.}

\begin{figure}[h]
    \centering
    \includegraphics[width=0.9\columnwidth]{images/LogisticBetterness.png}
    \vspace{-0.2cm}
    \caption{A synthetic example showing a possible benefit of logistic/cross entropy-based approximation of implicit bias in reducing the margin around a noisy point.}
    \label{fig:LogisticBetterness}
\vskip -0.1in
\end{figure}
